# Supplementary material for: CHAOS -- A Consistent Large-scale Database for Sigma-Profiles and Other Molecular Descriptors
Source: arXiv:2511.19002 ancillary file (2026-04-10)
Supplement: Supplementary file 1 [file SI_CHAOS.pdf]

# Supporting Information for 'CHAOS - A Consistent Large-scale Database for $\sigma$-Profiles and Other Molecular Descriptors'

Dominik Gond, Justus Arweiler, Thomas Specht, Hans Hasse, and Fabian Jirasek*

*Laboratory of Engineering Thermodynamics, RPTU Kaiserslautern, 67663 Kaiserslautern, Germany*

E-mail: fabian.jirasek@rptu.de

## Full list of properties within CHAOS

In the following, we give an overview of the entries of the CHAOS database, including all computed properties. In all cases, we introduce the names used in the database, followed by a brief description. In Figure 1, we visualize the distributions of the scalar properties in CHAOS in histogram representations.

### General information

- `CanonicalSMILES` – the canonical SMILES of the molecule, canonicalized with RDKit version `2024.3.1` in Python 3.12.4.
- `ID` – an internal identifier number for each molecule.
- `MolecularMass` – the molecular mass of the molecule, read from the Gaussian output file, provided as float scalar in atomic mass units u.

- `AtomList` – a list of all atoms comprising the molecule. The list holds dictionaries for each atom, with keys `index`, `element`, and `atomic_number`.
- `not_converged` – a Boolean flag indicating geometry optimization convergence of the molecule. If negative frequencies persisted after the second DFT cycle, the flag is set to `true`, and `false` otherwise.

## Structural properties

- `Coordinates` – the Cartesian coordinates in Gaussian's standard orientation. It is a list of lists (nested list), where each entry of the outer list is mapped to one atom, ordered according to `AtomList`. The order for the inner list, holding the Cartesian coordinate triple, is [$x$, $y$, $z$]. The unit of the coordinates is Å.
- `Coordniates_Input` – the Cartesian coordinates in Gaussian's input orientation. It is a list of lists (nested list), where each entry of the outer list is mapped to one atom, ordered according to `AtomList`. The order for the inner list, holding the Cartesian coordinate triple, is [$x$, $y$, $z$]. The unit of the coordinates is Å. The Gaussian input orientation could only be obtained for molecules with less than 52 atoms, including hydrogen atoms. If the input orientation is not obtainable, the JSON file entry is `None`. In these cases, please use `Coordinates` for access to Cartesian coordinates.
- `RotConst` – the rotational constants of the molecule, read from the Gaussian output file, in units of GHz. The value is a list holding the rotational constants ordered [$A$, $B$, $C$], following spectroscopic convention $A \geq B \geq C$. For linear molecules, a list with the solitary entry of $B$ is provided.
- `RotTemps` – the rotational temperatures of the molecule, read from the Gaussian output file, in units of K. The value is a list holding the rotational constants ordered [$T_A$, $T_B$, $T_C$], following spectroscopic convention $T_A \geq T_B \geq T_C$. For linear molecules, a list with the solitary entry of $T_B$ is provided.

- `PointGroup` – the Schönflies notation symbol for the molecule's point group, provided as string and read from the Gaussian output file, thus using the same symbols as Gaussian.

- `SymNumber` – the external symmetry number, read from the Gaussian output file, provided as integer.

## Electronic properties

- `Charge` – the molecule's total charge, calculated by RDKit, provided in units of elementary charges as integer.

- `Multiplicity` – the molecule's spin multiplicity $M_S$

$$M_S = 2S - 1, \tag{1}$$

  where $S$ is the molecule's total magnitude of electronic spin. Calculated by RDKit assuming a high-spin state for unpaired electrons obtained by RDKit's function `GetNumRadicalElectrons`. The multiplicity of oxygen was set to 3.

- `DipoleMoment` – the scalar magnitude of the molecule's dipole moment, read from the Gaussian output file, provided in units of D.

- `DipoleMoment_au` – the scalar magnitude of the molecule's dipole moment, read from the Gaussian output file, provided in atomic units, which are $e\,a_0$, where $e$ is the elementary charge and $a_0$ the Bohr radius.

- `DipoleMoment_SI` – the scalar magnitude of the molecule's dipole moment, read from the Gaussian output file, provided C m.

- `DipoleVec` – the vectorial dipole moment, read from the Gaussian output file, given in Gaussian's input orientation, provided as list ordered $[\mu_x, \mu_y, \mu_z]$ in units of D.

- DipoleVec_au – the vectorial dipole moment, read from the Gaussian output file, given in Gaussian's input orientation, provided as list ordered [$\mu_x$, $\mu_y$, $\mu_z$] in atomic units $e\,a_0$, where $e$ is the elementary charge and $a_0$ the Bohr radius.

- DipoleVec_SI – the vectorial dipole moment, read from the Gaussian output file, given in Gaussian's input orientation, provided as list ordered [$\mu_x$, $\mu_y$, $\mu_z$] in C m.

- QuadrupoleMoment – the scalar magnitude of the quadrupole matrix, read from the Gaussian output file, provided in units of D Å. It is calculated from the traceless quadrupole matrix's $\mathbf{Q}_{\text{tl}}$ diagonal elements.

$$Q = \frac{2}{3}\left((Q^{\text{tl}}_{xx})^2 + (Q^{\text{tl}}_{yy})^2 + (Q^{\text{tl}}_{zz})^2\right) \tag{2}$$

- QuadrupoleMat – the quadrupole matrix, read from the Gaussian output file, provided as dictionary with keys xx, yy, zz, xy, xz, and yz, in units of D Å.

- QuadrupoleMat_traceless – the traceless quadrupole matrix, read from the Gaussian output file, provided as dictionary with keys xx, yy, zz, xy, xz, and yz, in units of D Å.

- PolarMat – the dipole polarizability matrix, read from the Gaussian output file, provided as dictionary with keys xx, yy, zz, xy, xz, and yz, in units of $(a_0)^3$, where $a_0$ is the Bohr radius.

- PolarMat_SI – the dipole polarizability matrix, read from the Gaussian output file, provided as dictionary with keys xx, yy, zz, xy, xz, and yz, in $C^2\,m^2\,J^{-1}$.

- PolarMat_esu – the dipole polarizability matrix, read from the Gaussian output file, provided as dictionary with keys xx, yy, zz, xy, xz, and yz, in $cm^{-3}$.

- PolarIso – the dipole polarizability matrix's isotropic average $\alpha_{\text{iso}}$, read from the

Gaussian output file, for which

$$\alpha_{\text{iso}} = \frac{1}{3}\left(\alpha_{xx} + \alpha_{yy} + \alpha_{zz}\right) \tag{3}$$

applies. It is given in units of $(a_0)^3$, where $a_0$ is the Bohr radius.

- `PolarIso_SI` – the dipole polarizability matrix's isotropic average $\alpha_{\text{iso}}$, read from the Gaussian output file, for which equation 3 applies, in $\mathrm{C^2\,m^2\,J^{-1}}$.

- `PolarIso_esu` – the dipole polarizability matrix's isotropic average $\alpha_{\text{iso}}$, read from the Gaussian output file, for which equation 3 applies, in $\mathrm{cm^{-3}}$.

- `PolarAniso` – the dipole polarizability matrix's anisotropy $\alpha_{\text{aniso}}$, read from the Gaussian output file, for which

$$\alpha_{\text{aniso}} = \sqrt{\frac{1}{2}\left[\left(\alpha_{xx} - \alpha_{yy}\right)^2 + \left(\alpha_{yy} - \alpha_{zz}\right)^2 + \left(\alpha_{zz} - \alpha_{xx}\right)^2\right]} \tag{4}$$

applies. It is given in units of $(a_0)^3$, where $a_0$ is the Bohr radius.

- `PolarAniso_SI` – the dipole polarizability matrix's anisotropy $\alpha_{\text{aniso}}$, read from the Gaussian output file, for which equation 4 applies, in $\mathrm{C^2\,m^2\,J^{-1}}$.

- `PolarAniso_esu` – the dipole polarizability matrix's anisotropy $\alpha_{\text{aniso}}$, read from the Gaussian output file, for which equation 4 applies, in $\mathrm{cm^{-3}}$.

- `PartChargeMulliken` – atom-wise Mulliken partial charges, read from the Gaussian output file, provided as list in units of elementary charges.

- `PartChargeAPT` – atom-wise APT partial charges, read from the Gaussian output file, provided as list in units of elementary charges.

- `PartChargeMullikenHeavy` – list of Mulliken partial charges for heavy atoms, with the charges of the attached hydrogen atoms added to the corresponding heavy atom.

It is read from the Gaussian output file, provided in units of elementary charges.

- `PartChargeAPTHeavy` – list of APT partial charges for heavy atoms, with the charges of the attached hydrogen atoms added to the corresponding heavy atom. It is read from the Gaussian output file, provided in units of elementary charges.

- `SCFEnergy` – the self-consistent field energy of the molecule, read from the Gaussian output file, provided as float scalar in units of H. Please note that the energetic reference state in quantum-chemical calculations is defined as free electrons and atomic cores at an infinite distance from each other.

- `HOMOEnergy` – the orbital energy of the highest occupied molecular orbital (HOMO), read from the Gaussian output file, provided as float scalar in units of H.

- `LUMOEnergy` – the orbital energy of the lowest unoccupied molecular orbital (LUMO), read from the Gaussian output file, provided as float scalar in units of H.

- `HLG` – the HOMO-LUMO gap, which is the energetic difference between the HOMO and LUMO energy, provided as float scalar in units of eV.

- `HLG_Hartree` – the HOMO-LUMO gap, which is the energetic difference between the HOMO and LUMO energy, provided as float scalar in units of H.

## Vibrational properties

- `Frequencies` – the harmonic frequencies, read from the Gaussian output file, provided as list of floats in units of $\mathrm{cm}^{-1}$. Please note that the list's length depends on the number of atoms in a molecule. For a molecule with $N$ atoms, there are $3N - F$ harmonic frequencies, with $F = 5$ for linear molecules and $F = 6$ otherwise.

- `IRIntensities` – the corresponding IR intensities of the harmonic frequencies, read from the Gaussian output file, provided as list of floats in units of $\mathrm{km\,mol}^{-1}$. This list is of the same length as `Frequencies`.

- ForceConstants – the corresponding force constants of the harmonic frequencies, read from the Gaussian output file, provided as list of floats in units of mDyne mol$^{-}$1. This list is of the same length as Frequencies.

- ReducedMasses – the corresponding reduced masses of the harmonic frequencies, provided as list of floats in units of atomic units u. This list is of the same length as Frequencies.

- ZPE – the zero-point energy of the molecule, read from the Gaussian output file, provided as float scalar in units of J mol$^{-1}$. Please note that this energy does not account for deviations arising from the anharmonicity of real frequencies. To address this, we recommend scaling the molecular frequencies by a factor of 0.95461, as detailed in reference.[1]

- HeatCap – the molar isochoric heat capacity of the molecule at 298 K, read from the Gaussian output file, provided as float scalar in units of cal mol$^{-1}$ K$^{-1}$. Please note that this heat capacity does not account for deviations arising from the anharmonicity of real frequencies. To address this, we recommend scaling the molecular frequencies by a factor of 0.95461, as detailed in reference.[1]

- Entropy – the absolute entropy of the molecule at 298 K, read from the Gaussian output file, provided as float scalar in units of cal mol$^{-1}$ K$^{-1}$. Please note that this entropy does not account for deviations arising from the anharmonicity of real frequencies. To address this, we recommend scaling the molecular frequencies by a factor of 0.95461, as detailed in reference.[1]

- E_Thermal – the thermal energy of the molecule at 298 K, read from the Gaussian output file, provided as float scalar in units of kcal mol$^{-1}$. Please note that this energy does not account for deviations arising from the anharmonicity of real frequencies. To address this, we recommend scaling the molecular frequencies by a factor of 0.95461,

as detailed in reference.[1]

## NMR properties

- `ShieldIso` – the atom-wise isotropy of the shielding tensor, read from the Gaussian output file, provided as list in units of ppm.
- `ShieldAniso` – the atom-wise anisotropy of the shielding tensor, read from the Gaussian output file, provided as list in units of ppm.
- `SuscDia` – the diamagnetic susceptibility tensors, read from the Gaussian output file, provided as dictionary with keys `xx`, `yy`, `zz`, `xy`, `xz`, and `yz` in units of $\alpha^2 \, {a_0}^3$, where $\alpha$ is the fine-structure constant and $a_0$ is the Bohr radius.
- `SuscPara` – the paramagnetic susceptibility tensors, read from the Gaussian output file, provided as dictionary with keys `xx`, `yy`, `zz`, `xy`, `xz`, and `yz` in units of $\alpha^2 \, {a_0}^3$, where $\alpha$ is the fine-structure constant and $a_0$ is the Bohr radius.
- `SuscDiaIso` – the isotropic average of the diamagnetic susceptibility tensors, read from the Gaussian output file, provided as float scalar in units of $\alpha^2 \, {a_0}^3$, where $\alpha$ is the fine-structure constant and $a_0$ is the Bohr radius.
- `SuscParaIso` – the isotropic average of the paramagnetic susceptibility tensors, read from the Gaussian output file, provided as float scalar in units of $\alpha^2 \, {a_0}^3$, where $\alpha$ is the fine-structure constant and $a_0$ is the Bohr radius.

## Solvation properties

- `CavArea` – the area of the cavity surface, read from the Gaussian output file, provided as float scalar in units of $(a_0)^2$.
- `CavVol` – the volume of the cavity, read from the Gaussian output file, provided as float scalar in units of $(a_0)^3$.

- `CavSegments` – the number of segments comprising the cavity, read from the Gaussian output file, provided as integer.

- `SCFCOSMOEnergy` – the self-consistent field energy of the molecule inside the cavity, read from the Gaussian output file, provided as float scalar in units of H. Please note that the energetic reference state in quantum-chemical calculations is defined as free electrons and atomic cores at an infinite distance from each other. Also, consider that this energy is the internal energy and should not be mistaken with the Gibbs energy.

- `DielectricCorr` – the dielectric correction to the molecule-cavity system, which is the interaction between the polarized solute and the solvent, read from the Gaussian output file, provided as float scalar in units of kcal mol$^{-}$1.

- `CavEnergy` – the energy contribution of the cavity to the total energy of the molecule-cavity system, read from the Gaussian output file, provided as float scalar in units of kcal mol$^{-}$1.

- `DispersionEnergy` – the dispersion contribution of the molecule-cavity system, read from the Gaussian output file, provided as float scalar in units of kcal mol$^{-}$1.

- `PauliRepulsion` – the Pauli repulsion contribution of the molecule-cavity system, read from the Gaussian output file, provided as float scalar in units of kcal mol$^{-}$1.

- `Sigma_NHB` – the normalized $\sigma$-profile for non-hydrogen bonding atoms in units of Å$^2$, calculated according to NIST's COSMO-SAC-dsp protocol. The bins are located at segment charges between -0.025 and 0.025 $e$/Åin steps of 0.001 $e$/Å.

- `Sigma_OH` – the normalized $\sigma$-profile for hydrogen bonding atoms within hydroxyl groups, in units of Å$^2$, calculated according to NIST's COSMO-SAC-dsp protocol. The bins are located at segment charges between -0.025 and 0.025 $e$/Åin steps of 0.001 $e$/Å.

- `Sigma_OT` – the normalized $\sigma$-profile for hydrogen bonding atoms within other groups than hydroxyl groups, in units of Å$^2$, calculated according to NIST's COSMO-SAC-dsp protocol. The bins are located at segment charges between -0.025 and 0.025 $e$/Åin steps of 0.001 $e$/Å.

- `Sigma_total` – the unnormalized total $\sigma$-profile, provided in units of Å$^2$, calculated according to NIST's COSMO-SAC-dsp protocol. The bins are located at segment charges between -0.025 and 0.025 $e$/Åin steps of 0.001 $e$/Å.

- `Norm_Sigma_total` – the integral of the total $\sigma$-profile, which equals `CavArea` in units of Å$^2$.

- `Fraction_PartSigmas` – the proportions of the partial $\sigma$-profiles to the total $\sigma$-profile, provided as list, ordered [NHB, OH, OT].

- `SegmentList` – detailed output, usable for creating $\sigma$-profiles, read from the Gaussian output file, provided as a list of lists (nested list), where every entry of the outer list is mapped to one segment. The inner lists hold, in the following order, the sequential segment number, the index of the segment's atom, the $x$ coordinate of the segment, the $y$ coordinate of the segment, the $z$ coordinate of the segment, the charge of the segment, the area of the segment, the surface charge density of the segment, and the segment's potential. These data are only provided in the molecule-specific JSON files.

## Visualization of scalar properties in CHAOS

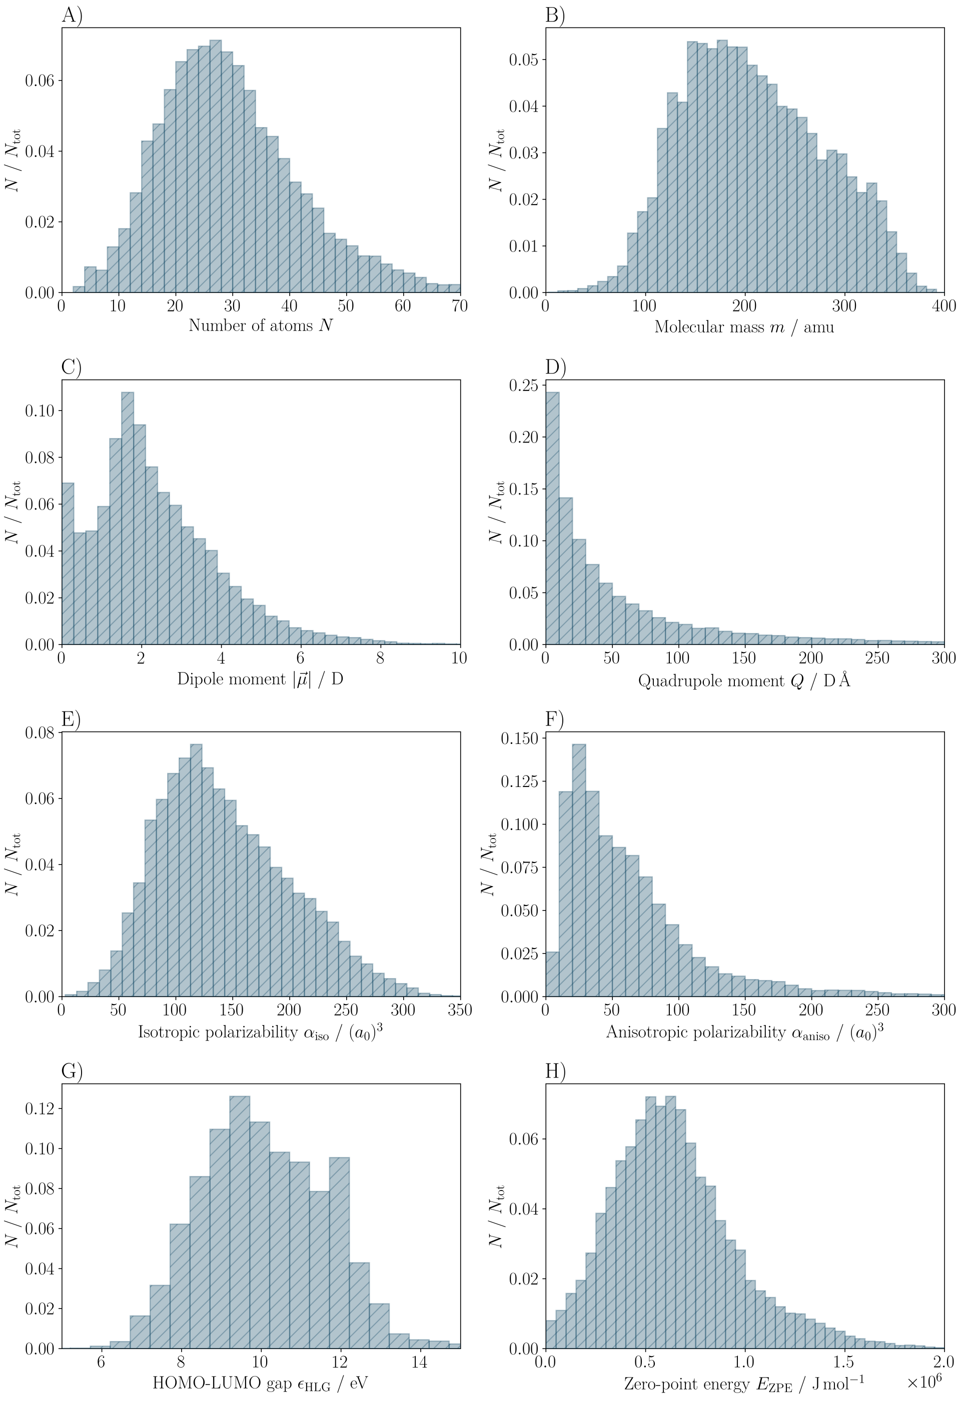


Figure 1: Overview of the diversity of the molecules' scalar properties included in the CHAOS database. Panel A) shows the number of atoms, B) the molecular mass, C) the dipole moment, D) the quadrupole moment, E) the isotropic polarizability, F) the anisotropic polarizability, G) the HOMO-LUMO gap, H) the zero-point energy. The number of molecules in a given class is reported as a fraction of the total number of molecules $N_{\mathrm{tot}} = 53\,091$ in all panels.

# Calculation of ideal-gas properties

Ideal-gas properties can be derived by applying standard relations from statistical thermodynamics within the rigid-rotor-harmonic-oscillator (RRHO) approximation. The ideal-gas Helmholtz energy is given as

$$A_{\mathrm{id}} = -k_{\mathrm{B}} T \ln\left(Q_{\mathrm{id}}\right) \tag{5}$$

where $k_{\mathrm{B}}$ is the Boltzmann constant, $T$ is the absolute temperature, and $Q_{\mathrm{id}}$ is the partition function of the ideal gas within the RRHO approximation. The partition function for $N$ indistinguishable molecules can be described as

$$Q_{\mathrm{id}} = \frac{q_{\mathrm{id}}^{N}}{N!} \tag{6}$$

Here, $q_{\mathrm{id}}$ is the partition function of a single molecule, which comprises of partition functions of the given degrees of freedom

$$q_{\mathrm{id}} = q_{\mathrm{elec}} \cdot q_{\mathrm{vib}} \cdot q_{\mathrm{rot}} \cdot q_{\mathrm{trans}} \tag{7}$$

where $q_{\mathrm{elec}}$ is the electronic, $q_{\mathrm{vib}}$ the vibrational, $q_{\mathrm{rot}}$ the rotational, and $q_{\mathrm{trans}}$ the translational part of the partition function. The electronic partition function is obtained from the electronic spin of the molecule, the vibrational partition function from the harmonic frequencies, the rotational partition function from the rotational constants and the external symmetry number, and the translational partition function from the molecular mass. These partition functions are obtained by

$$q_{\text{elec}} = 2s + 1 \tag{8}$$

$$q_{\text{vib}} = \prod_{i=1}^{F} \exp\left(\frac{-hc\nu_i}{2k_{\text{B}}T}\right)\left[1 - \exp\left(\frac{-hc\nu_i}{k_{\text{B}}T}\right)\right]^{-1} \tag{9}$$

$$q_{\text{rot}} = \frac{\pi^{0.5}\left(k_{\text{B}}T\right)^{1.5}}{h^{1.5}\left(ABC\right)^{0.5}\sigma^{\text{sym}}} \tag{10}$$

$$q_{\text{trans}} = \left(\frac{2\pi m k_{\text{B}}T}{h^2}\right)V \tag{11}$$

with the electronic spin $s$, the number of vibrational degrees of freedom $F$, Planck's Constant $h$, the vibrational frequency of the $i$th mode $\nu_i$, the rotational constants $A$, $B$, and $C$, the external symmetry number $\sigma^{\text{sym}}$, the molecular mass $m$, and the volume $V$. For linear molecules, the rotational partition function is defined as

$$q_{\text{rot,lin}} = \frac{k_{\text{B}}T}{hB\sigma^{\text{sym}}} \tag{12}$$

The ideal-gas Helmholtz energy serves as a fundamental potential from which other thermodynamic ideal-gas properties can be derived. For example, the molar isochoric heat capacity is defined as

$$c_{\text{v,id}} = -T\left(\frac{\partial^2 a_{\text{id}}}{\partial T^2}\right)_v = 2RT\left(\frac{\partial \ln q_{\text{id}}}{\partial T}\right)_v + RT^2\left(\frac{\partial^2 \ln q_{\text{id}}}{\partial T^2}\right)_v \tag{13}$$

In the RRHO approximation, the total isochoric heat capacity of a closed-shell ($s = 0$) molecule is thus obtained as the sum of translational, rotational, and vibrational contributions

$$c_{\text{v,id}} = c_{\text{v,trans}} + c_{\text{v,rot}} + c_{\text{v,vib}} \tag{14}$$

where the individual terms are given by

$$c_{\mathrm{v,trans}} = \frac{3}{2}R \tag{15}$$

$$c_{\mathrm{v,rot}} = \begin{cases} R & \text{for linear molecules} \\ \frac{3}{2}R & \text{for nonlinear molecules} \end{cases} \tag{16}$$

$$c_{\mathrm{v,vib}} = R\sum_{i=1}^{F}\left(\frac{h\nu_i}{k_{\mathrm{B}}T}\right)^2 \frac{\exp\left(\frac{h\nu_i}{k_{\mathrm{B}}T}\right)}{\left[\exp\left(\frac{h\nu_i}{k_{\mathrm{B}}T}\right) - 1\right]^2} \tag{17}$$

# Implementation details of workflow

## Initial molecular geometry generation

All steps described in the main section "Generation of initial molecular geometries" were performed using RDKit version `2024.3.1` in Python 3.12.4. The workflow converts molecular structures from the Dortmund Data Bank (DDB),[2] given within MOL files, into force-field-optimized structures, suitable for subsequent semi-empirical refinement. The corresponding RDKit function calls are listed below for reproducibility

### Import and canonicalization

The original MOL file geometry from the DDB where read with `Chem.MolFromMolFile` and transformed into a canonical SMILES with `Chem.MolToSmiles`. The SMILES were then reimported to a `Mol object` via `Chem.MolFromSmiles`. Hydrogen atoms were added explicitly using `Chem.AddHs`.

### Conformer generation

From the obtained `Mol object`, a 3D ensemble of 300 conformers was generated with `AllChem.EmbedMultipleConfs` using the ETKDG[3] algorithm.

### Energy filtering

Conformer energies were evaluated with the Universal Force Field (UFF)[4] using `AllChem.UFFGetMoleculeForceField`. The conformers were sorted in ascending energy, and only those differing by more than $\Delta E_{\text{cut}} = 1.0\,\text{kcal mol}^{-1}$ from previously accepted structures were retained. This threshold efficiently removes near-degenerate geometries while preserving thermally accessible minima.

### Final UFF optimization

Each retained conformer was re-optimized with `AllChem.UFFGetMoleculeForceField` and the structure with the lowest UFF energy was selected as the final geometry for the subsequent semi-empirical conformer refinement step.

## Semi-empirical conformer refinement

This section provides the technical details of the semi-empirical refinement step described in the main text. Each molecular geometry obtained from the force-field conformer search was used as the starting point for an exhaustive conformational search with CREST (conformer–rotamer sampling tool)[5](version `2.12`) using the GFN2-xTB[6] (Geometry, Frequency, Noncovalent, extended tight binding) Hamiltonian. We set the CREST energy window parameter to `ewin` $= 1.0\,\text{kcal}\,\text{mol}^{-1}$, since we focused exclusively on the most relevant low-energy structures. This narrow window keeps CREST's Generic Structure Crossing (GC) step from exploding in size, which in turn limits CPU time and prevents the otherwise dramatic increase in memory requirements for larger molecules. CREST reports a ranked list of unique minima; only the conformer with the lowest energy was forwarded to the subsequent DFT stage. The exact command-line input is shown in Listing 1.

```
crest <rdkit.xyz_path> --T 6 --gfn2 --ewin 1
```

Listing 1: Command structure for CREST jobs used in the workflow employed in this work. The option `-T` requests 6 CPU cores, `-gfn2` requests the use of the GFN2-xTB Hamiltonian, and `-ewin` specifies the energy window parameter of CREST.

## High-level quantum-chemical calculations

This section provides the technical details of the DFT[7] workflow described in the main text. All high-level calculations were performed with Gaussian 16.[8] The $\omega$B97X-D functional[9] in combination with the def2-TZVP basis set[10] was used throughout. First, the geometry of each component obtained from CREST was optimized. Geometry optimization was followed by a harmonic frequency analysis; if a saddle point was detected (indicated by imaginary modes), the structure was displaced along the most negative eigenmode and optimized again. Should an imaginary frequency persist after this second optimization, the workflow was completed, and the corresponding entry in the database was marked with the flag `not_converged = True`, which occurred for only 369 molecules (0.69%) in the CHAOS database. Subsequently, NMR shielding tensors were computed with the `NMR=GIAO` keyword,[11] followed by a single-point C-PCM[12,13] (`SCRF=COSMORS`) calculation performed *without* further geometry relaxation to retain the gas-phase minimum. An example Gaussian 16 input file with all keywords is shown in Listing 2.

```
%Mem=...
%NProcShared=...
%chk=...
# opt def2TZVP wB97XD IOp(1/6=100) symm=loose IOp(2/16=3) IOp(2/17=3)

water_dft

0 1
```

```
O        -0.22832      2.94749      0.00000
H         0.74168      2.94749      0.00000
H        -0.55165      2.36236      0.70283
--link1--
%Mem=...
%NProcShared=...
%chk=...
# freq polar geom=Allcheck def2TZVP wB97XD IOp(1/6=100) symm=loose IOp(2/16=3)
    IOp(2/17=3)

--link1--
%Mem=...
%NProcShared=...
%chk=...
# nmr=(giao,PrintEigenvectors,Susceptibility) geom=Allcheck def2TZVP wB97XD IOp
    (1/6=100) symm=loose IOp(2/16=3) IOp(2/17=3)

--link1--
%Mem=...
%NProcShared=...
%chk=...
#p scrf=COSMORS geom=Allcheck def2TZVP wB97XD

water_dft.cosmo
```

Listing 2: Gaussian input file for water used for the DFT workflow of this work. The file is structured into four blocks: optimization called with the `opt` keyword, frequency calculation called with the `freq` keyword, NMR calculations called with the `nmr` keyword, and C-PCM calculations called with the `scrf` keyword.

# Literature Cited


(1) Kesharwani, M. K.; Brauer, B.; Martin, J. M. Frequency and zero-point vibrational energy scale factors for double-hybrid density functionals (and other selected methods): can anharmonic force fields be avoided? *The Journal of Physical Chemistry A* **2015**, *119*, 1701–1714.

(2) Dortmund Data Bank , 2024. `www.ddbst.com`.

(3) Riniker, S.; Landrum, G. A. Better informed distance geometry: using what we know to improve conformation generation. *Journal of chemical information and modeling* **2015**, *55*, 2562–2574.

(4) Rappé, A. K.; Casewit, C. J.; Colwell, K.; Goddard III, W. A.; Skiff, W. M. UFF, a full periodic table force field for molecular mechanics and molecular dynamics simulations. *Journal of the American chemical society* **1992**, *114*, 10024–10035.

(5) Pracht, P.; Bohle, F.; Grimme, S. Automated exploration of the low-energy chemical space with fast quantum chemical methods. *Physical Chemistry Chemical Physics* **2020**, *22*, 7169–7192.

(6) Bannwarth, C.; Ehlert, S.; Grimme, S. GFN2-xTB—An accurate and broadly parametrized self-consistent tight-binding quantum chemical method with multipole electrostatics and density-dependent dispersion contributions. *Journal of chemical theory and computation* **2019**, *15*, 1652–1671.

(7) Kohn, W.; Sham, L. J. Self-consistent equations including exchange and correlation effects. *Physical review* **1965**, *140*, A1133.

(8) Frisch, M. J. et al. Gaussian~16 Revision C.01. 2016; Gaussian Inc. Wallingford CT.

(9) Chai, J.-D.; Head-Gordon, M. Systematic optimization of long-range corrected hybrid density functionals. *The Journal of chemical physics* **2008**, *128*.

(10) Weigend, F.; Ahlrichs, R. Balanced basis sets of split valence, triple zeta valence and quadruple zeta valence quality for H to Rn: Design and assessment of accuracy. *Physical Chemistry Chemical Physics* **2005**, *7*, 3297–3305.

(11) Ruud, K.; Helgaker, T.; Bak, K. L.; Jo/rgensen, P.; Jensen, H. J. A. Hartree–Fock limit magnetizabilities from London orbitals. *The Journal of chemical physics* **1993**, *99*, 3847–3859.

(12) Barone, V.; Cossi, M. Quantum calculation of molecular energies and energy gradients in solution by a conductor solvent model. *The Journal of Physical Chemistry A* **1998**, *102*, 1995–2001.

(13) Cossi, M.; Rega, N.; Scalmani, G.; Barone, V. Energies, structures, and electronic properties of molecules in solution with the C-PCM solvation model. *Journal of computational chemistry* **2003**, *24*, 669–681.
